# Supplementary material for: Localized Topological Simplification of Scalar Data
Source: arXiv:2009.00083 source file (2020-08-31)
Supplement: Supplementary file 1 [file 9_appendix.tex]

\begin{figure*}[!ht]

    \vspace{5em}
    \centering
    \adjustbox{width=\linewidth,center}{
    \input{figures/turbulence/turbulence.tex}
    }
    \vspace*{-1.5em}
    \mycaption{
    Level set based segmentation in an isotropic turbulence
simulation~\cite{openSciVisDataSets}.
    \jonasRevision{Initially, the segmentation contains a high number of small
features, which are progressively removed based on their vorticity (left to
right).}
    For these thresholds, LTS takes at most $1.79s$ to compute, and thus being
$27$ times faster than the baseline approach~\cite{tierny_vis12}.%
    }
    \vspace{-5em}
    \label{fig_turbulence}
\end{figure*}

\begin{figure*}[!ht]
    \adjustbox{width=\linewidth,center}{
    \input{./figures/ocean/ocean.tex}
    }
    \vspace*{-1.5em}
    \mycaption{Contour tree based vortex extraction in climate data (sea surface
    height), for increasing persistence thresholds.
    Clockwise (yellow) and counterclockwise (red)
    vortices are extracted by
    segmenting the regions corresponding to leaf arcs in the contour tree.
    The hierarchy (from left to
    right) progressively reveals 
    \julienRevision{the most persistent features}
    south of Australia.
    Pre-simplifying the data with the baseline approach~\cite{tierny_vis12} takes
    $1.22s$ while computing the contour-tree based segmentation
  ~\cite{gueunet_tpds19} takes $0.21s$. LTS requires only $0.06s$,
    resulting in an overall \emph{pipeline-speedup} of \speedup{5}.}
    \label{fig_ocean}
\end{figure*}
